# Supplementary material for: 3DRef: 3D Dataset and Benchmark for Reflection Detection in RGB and Lidar Data
Source: arXiv:2403.06538 source file (2024-03-11)
Supplement: Supplementary file 1 [file X_suppl.tex]

\clearpage
\setcounter{page}{1}
\maketitlesupplementary

\section*{Supplementary Material}

This document provides additional details and results for the paper ``3DRef: 3D Dataset and Benchmark for Reflection Detection in RGB and Lidar Data".
\subsection*{Additional Dataset Sequence Images}

Figures \ref{fig:seq1_images}-\ref{fig:seq3_images} provide additional visualizations of the multi-modal data across sequences in the 3DRef dataset. For each sequence, point clouds from the Ouster, Hesai, and Livox Lidars are shown, along with a labeled point cloud depicting the ground truth annotations. In each subfigure of Lidar pointcloud from (a) to (c), the point color means the return number, red represent the first return, green represent the second return and blue represent the third return.

\begin{figure}[ht]
\centering
\begin{subfigure}{0.95\linewidth}
\includegraphics[width=\linewidth]{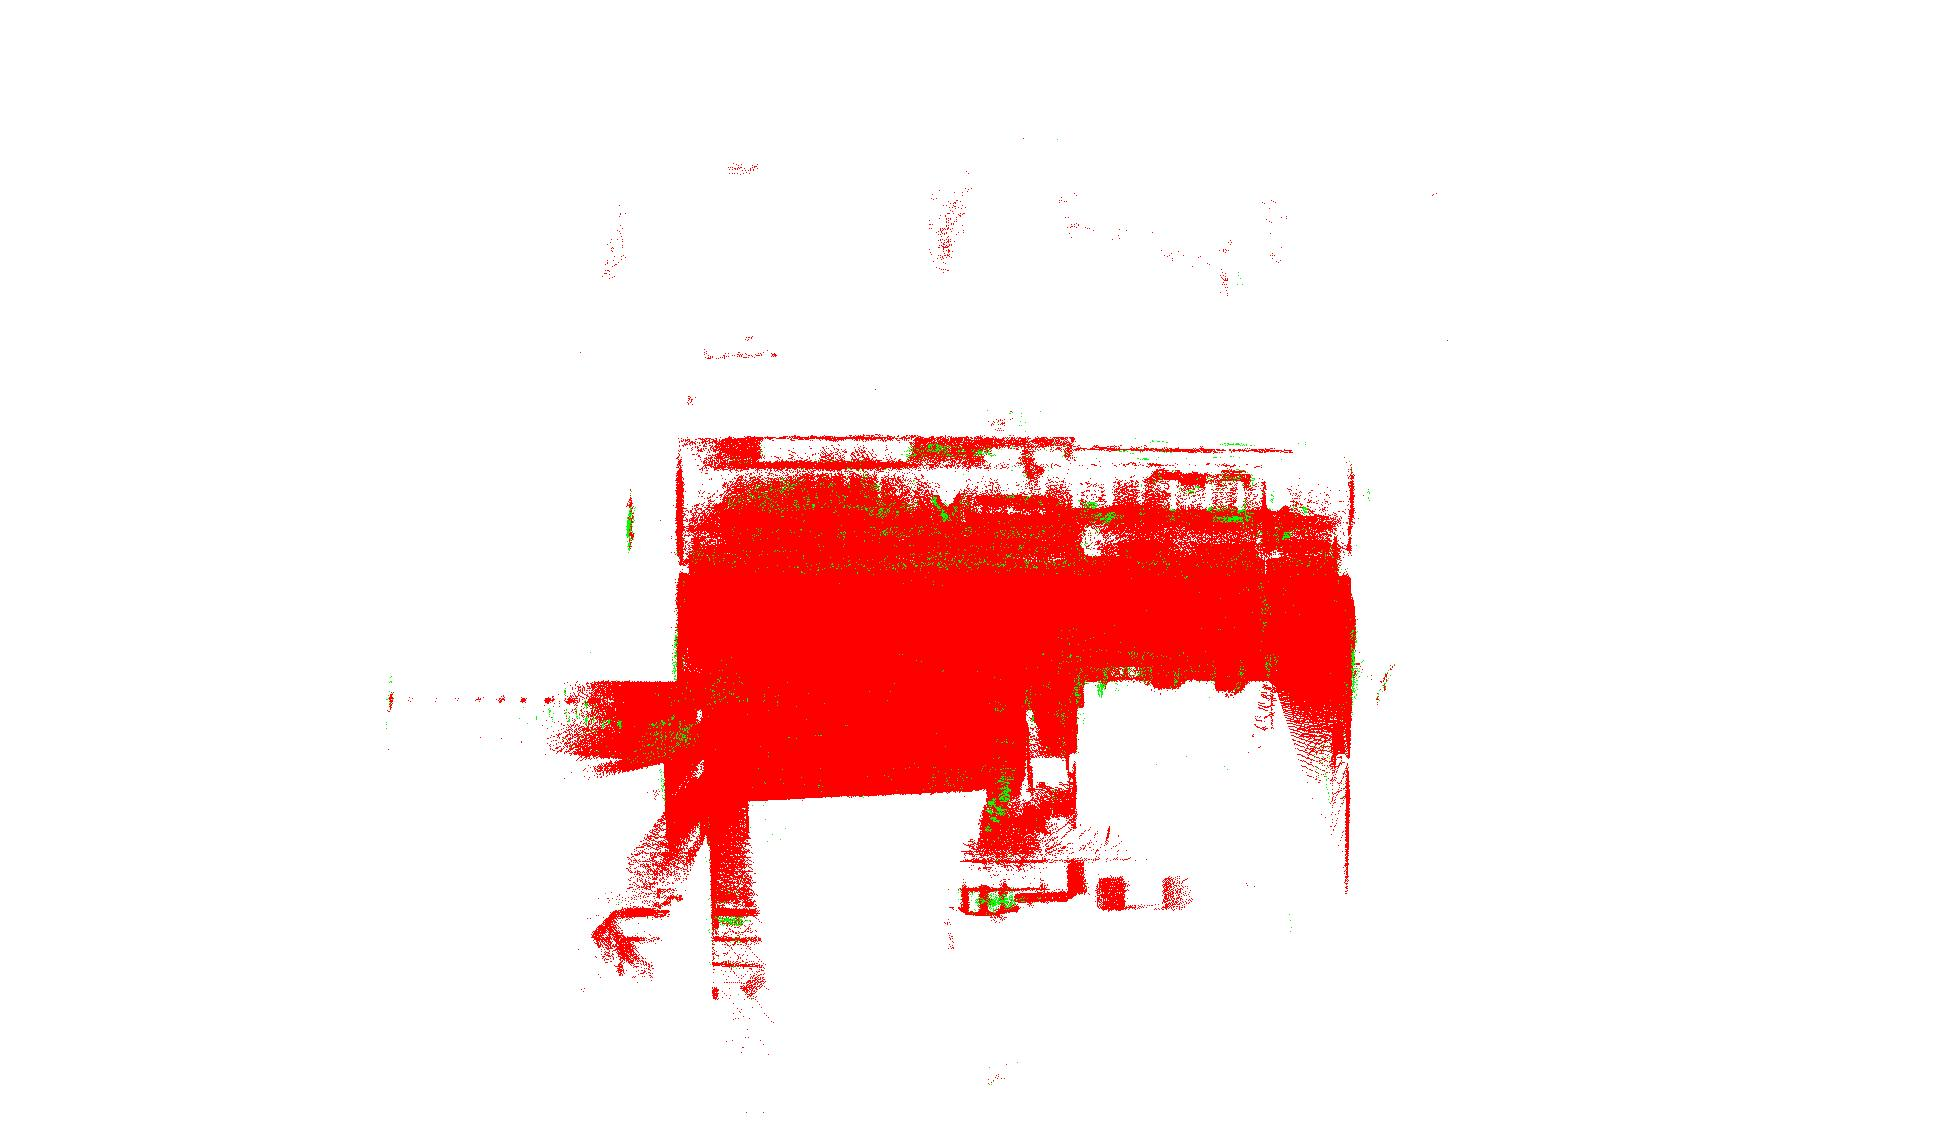}
\caption{Ouster}
\end{subfigure}
\begin{subfigure}{0.95\linewidth}
\includegraphics[width=\linewidth]{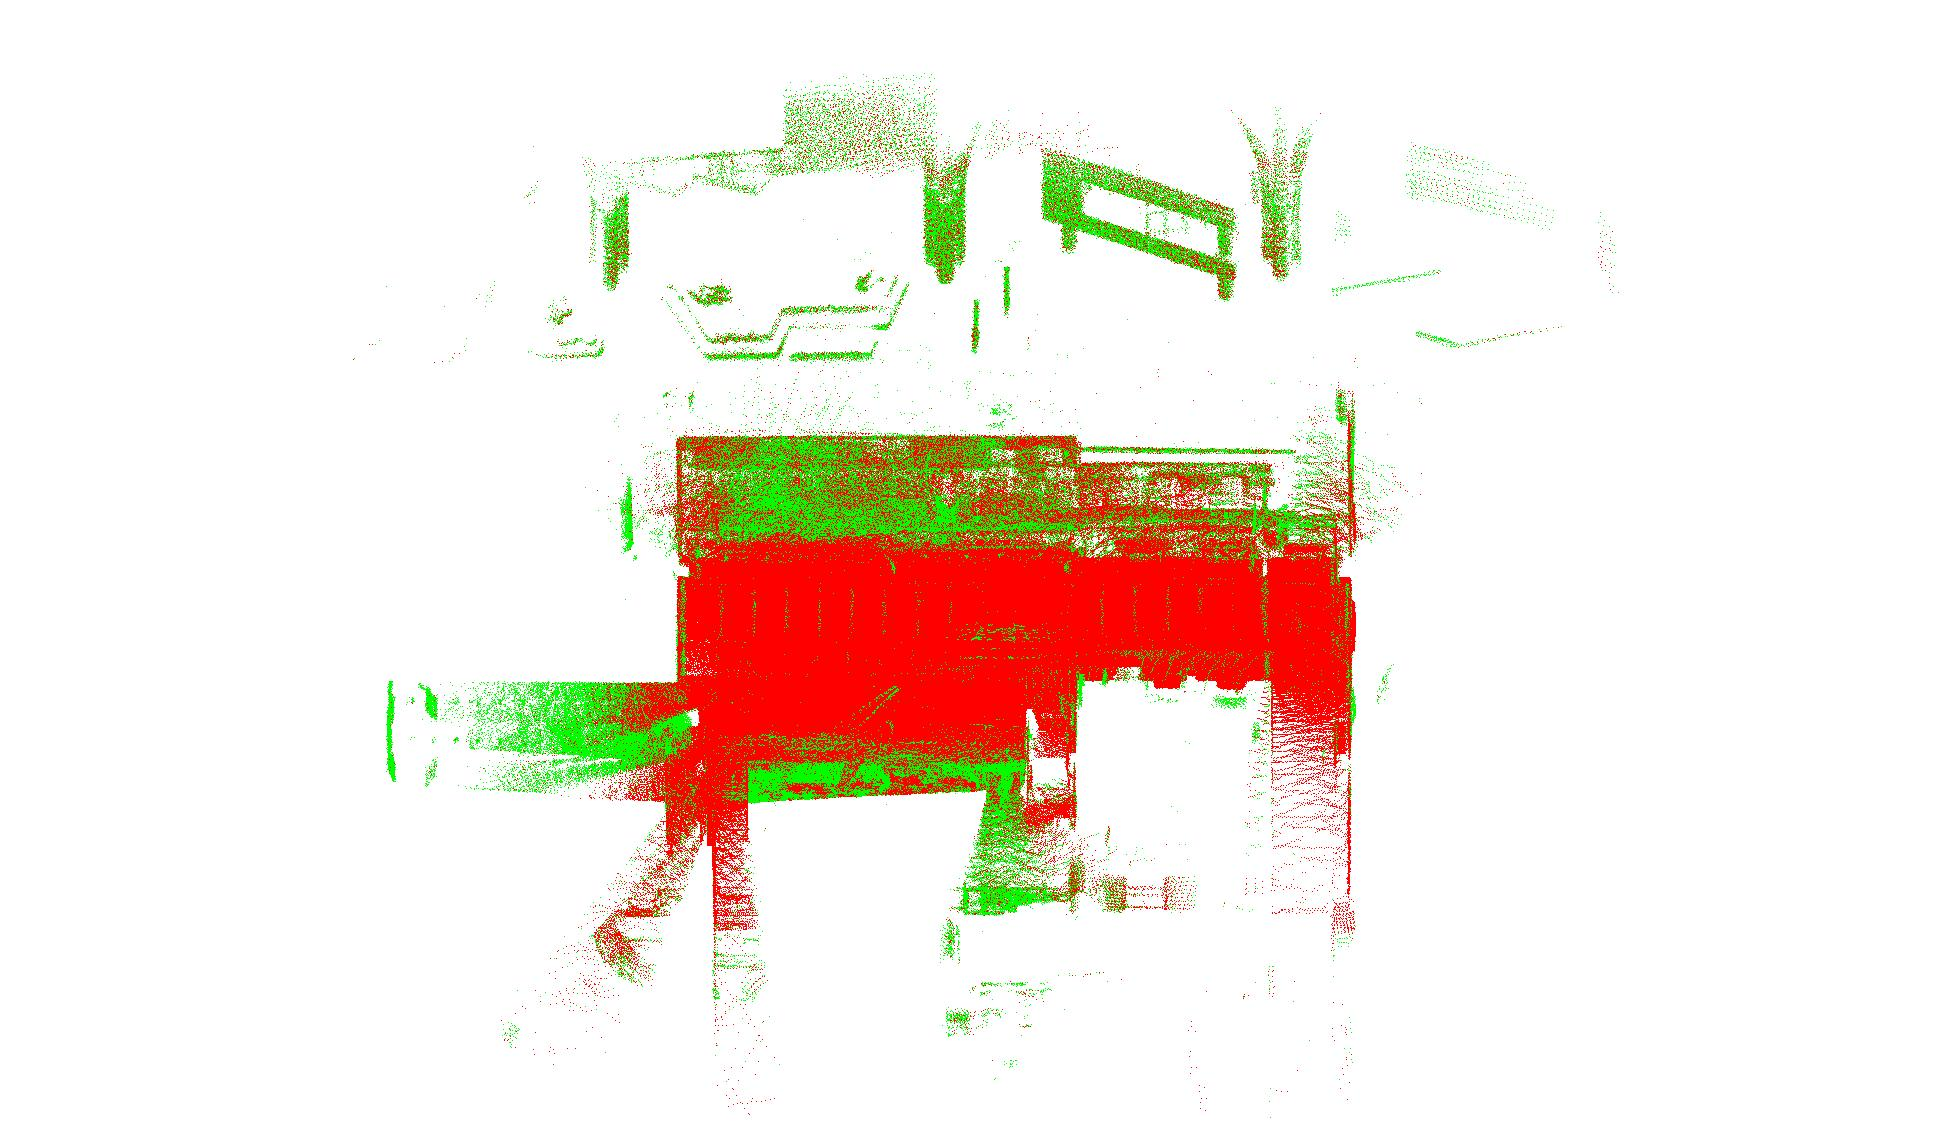}
\caption{Hesai}
\end{subfigure}
\begin{subfigure}{0.95\linewidth}
\includegraphics[width=\linewidth]{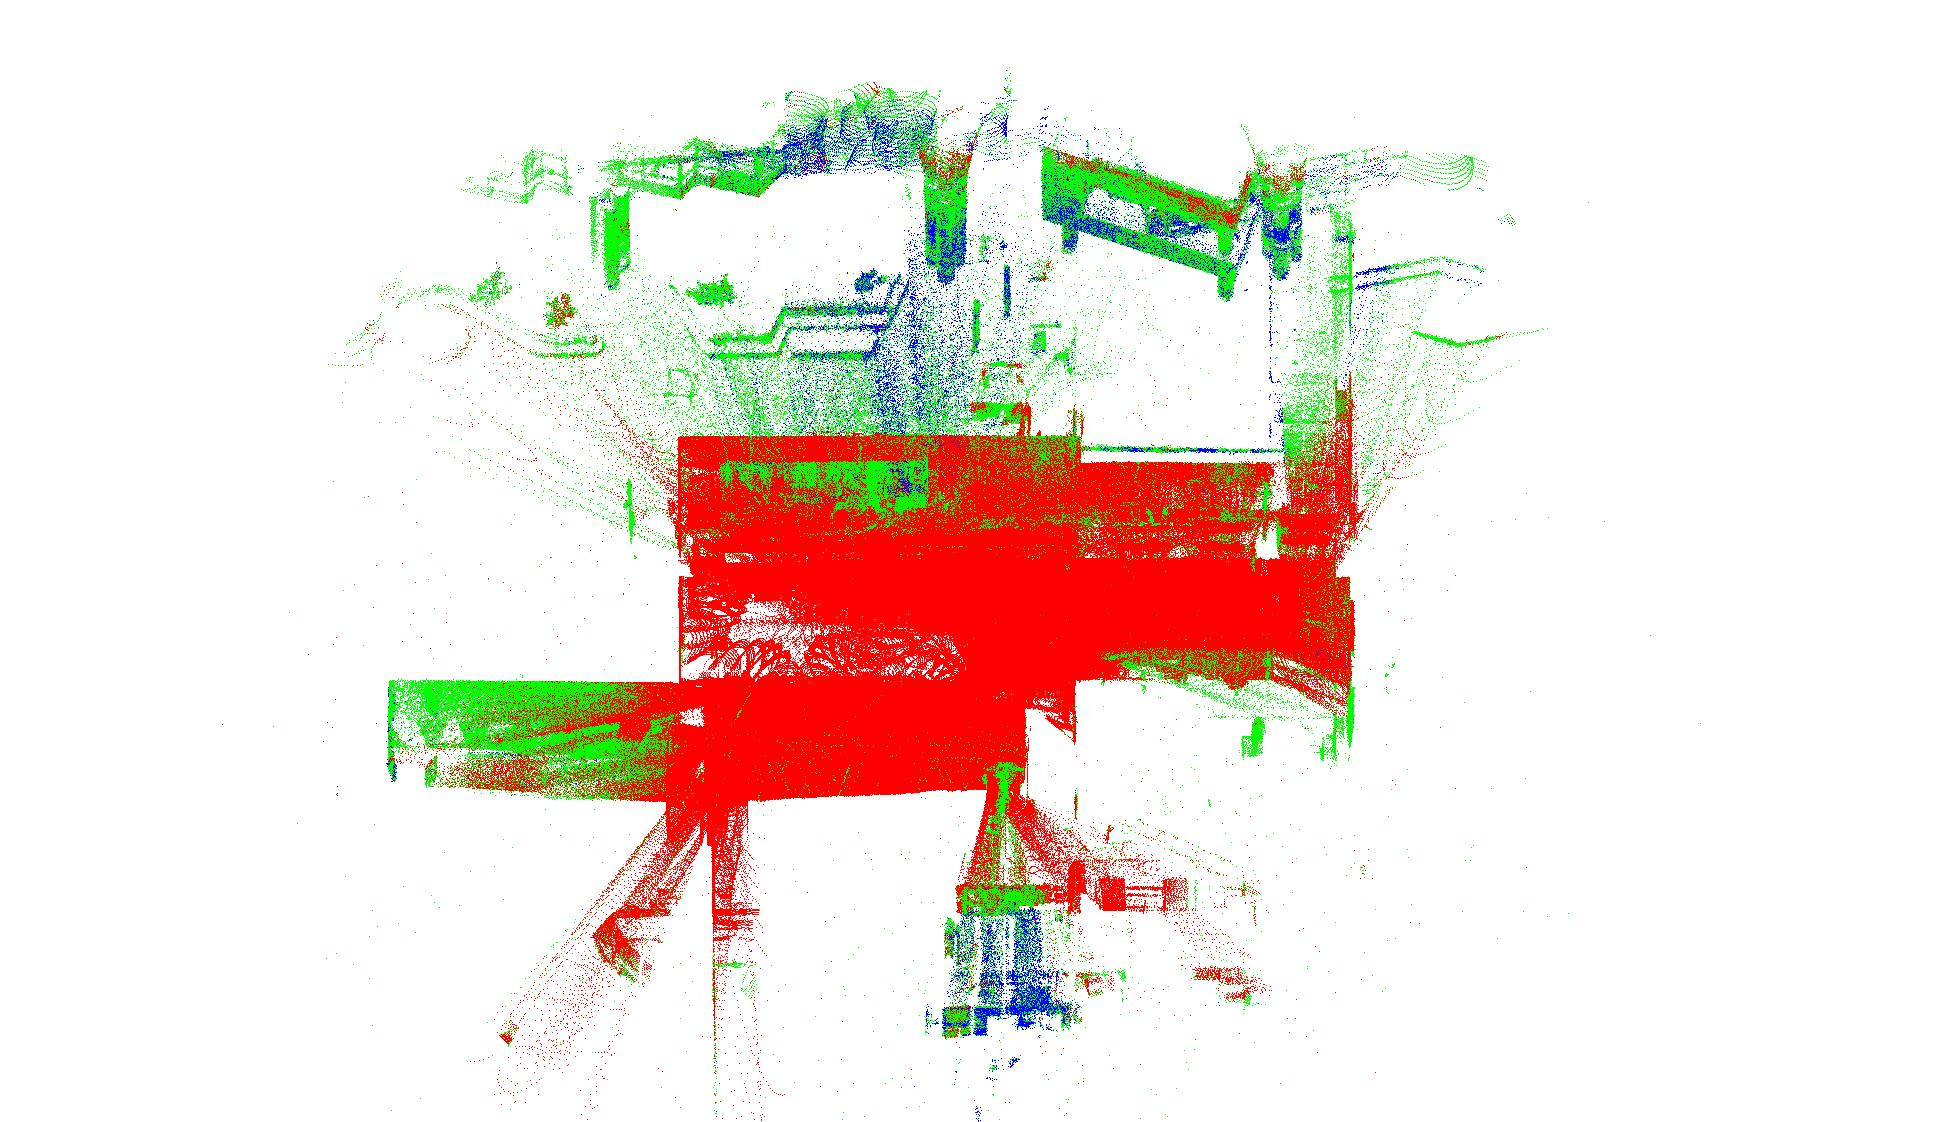}
\caption{Livox}

\end{subfigure}
\begin{subfigure}{0.95\linewidth}
\includegraphics[width=\linewidth]{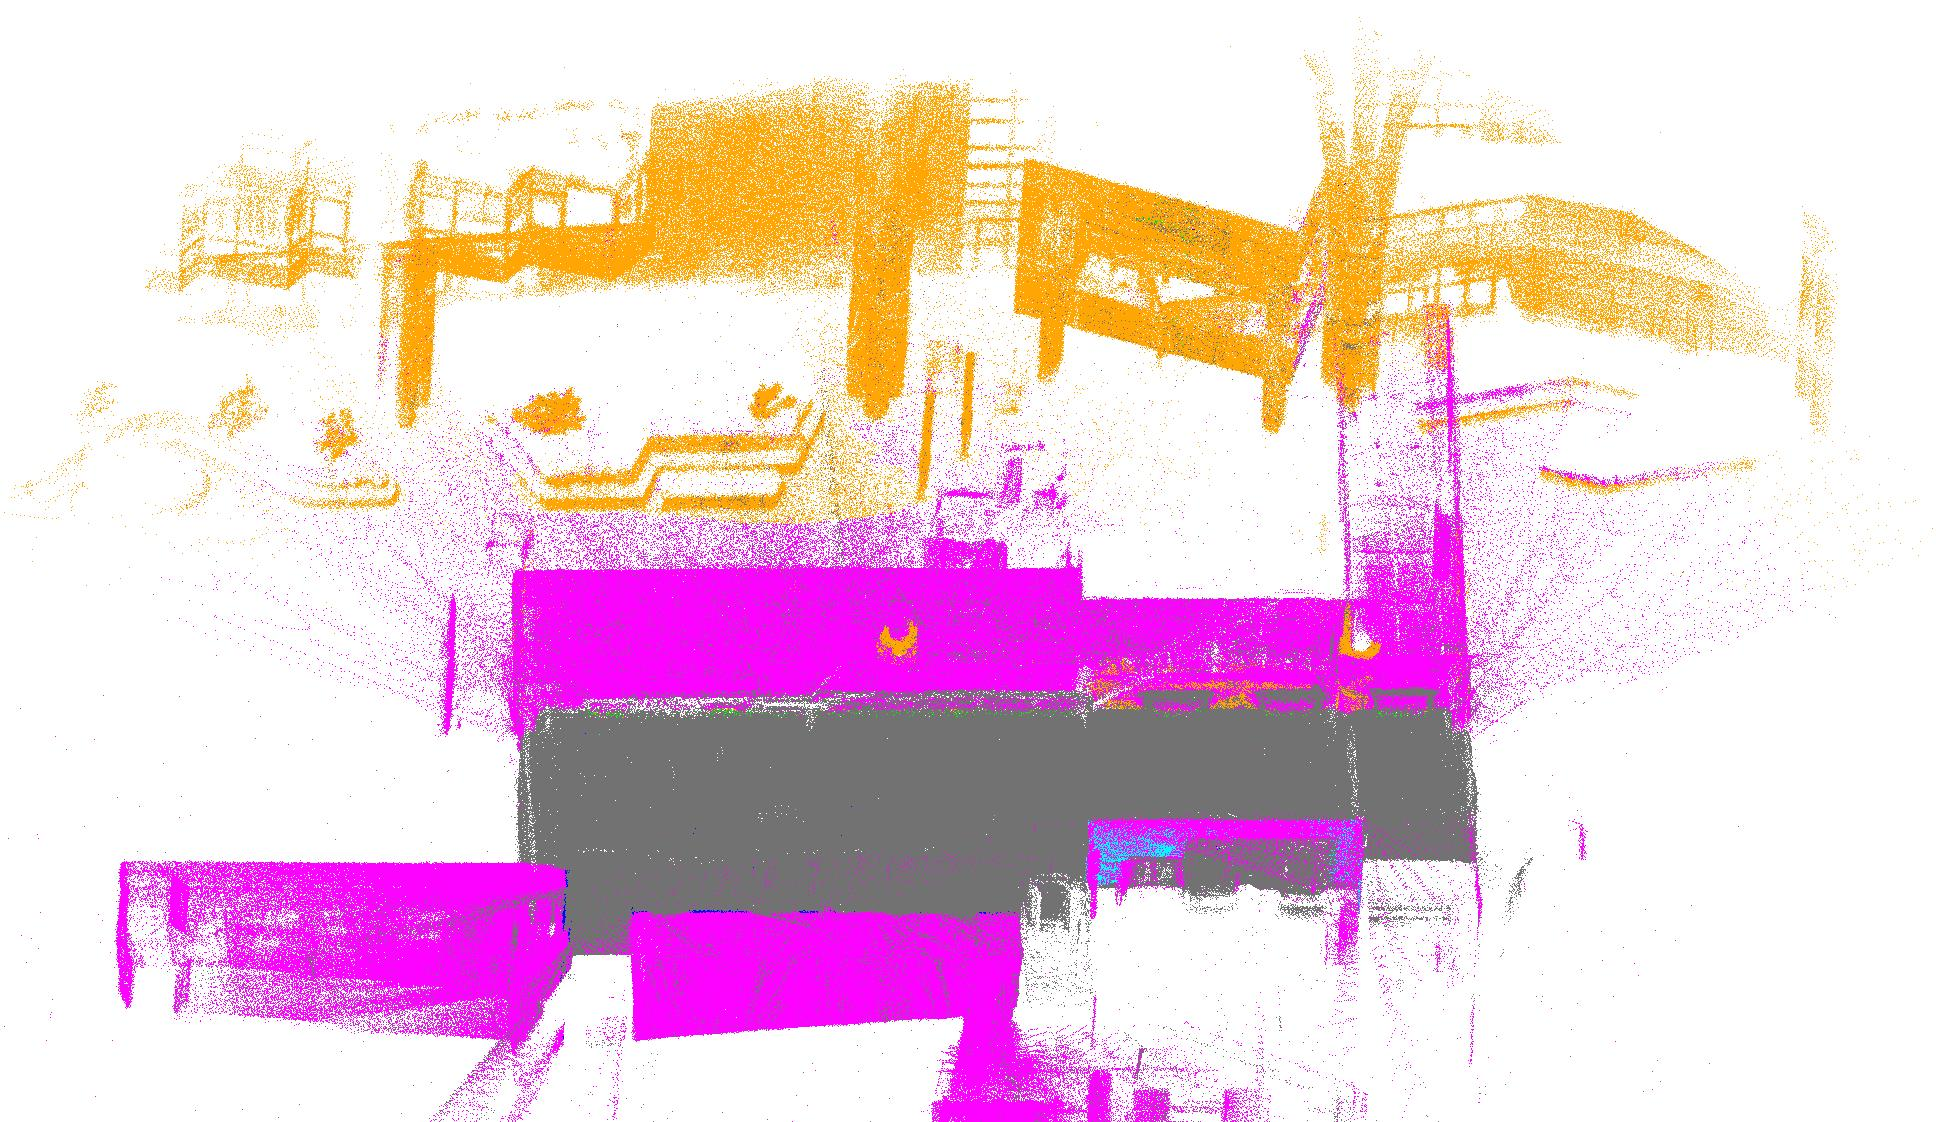}
\caption{Labels}
\end{subfigure}
\caption{Additional images from Sequence 1}
\label{fig:seq1_images}
\end{figure}

\begin{figure}[ht]
\centering
\begin{subfigure}{0.95\linewidth}
\includegraphics[width=\linewidth]{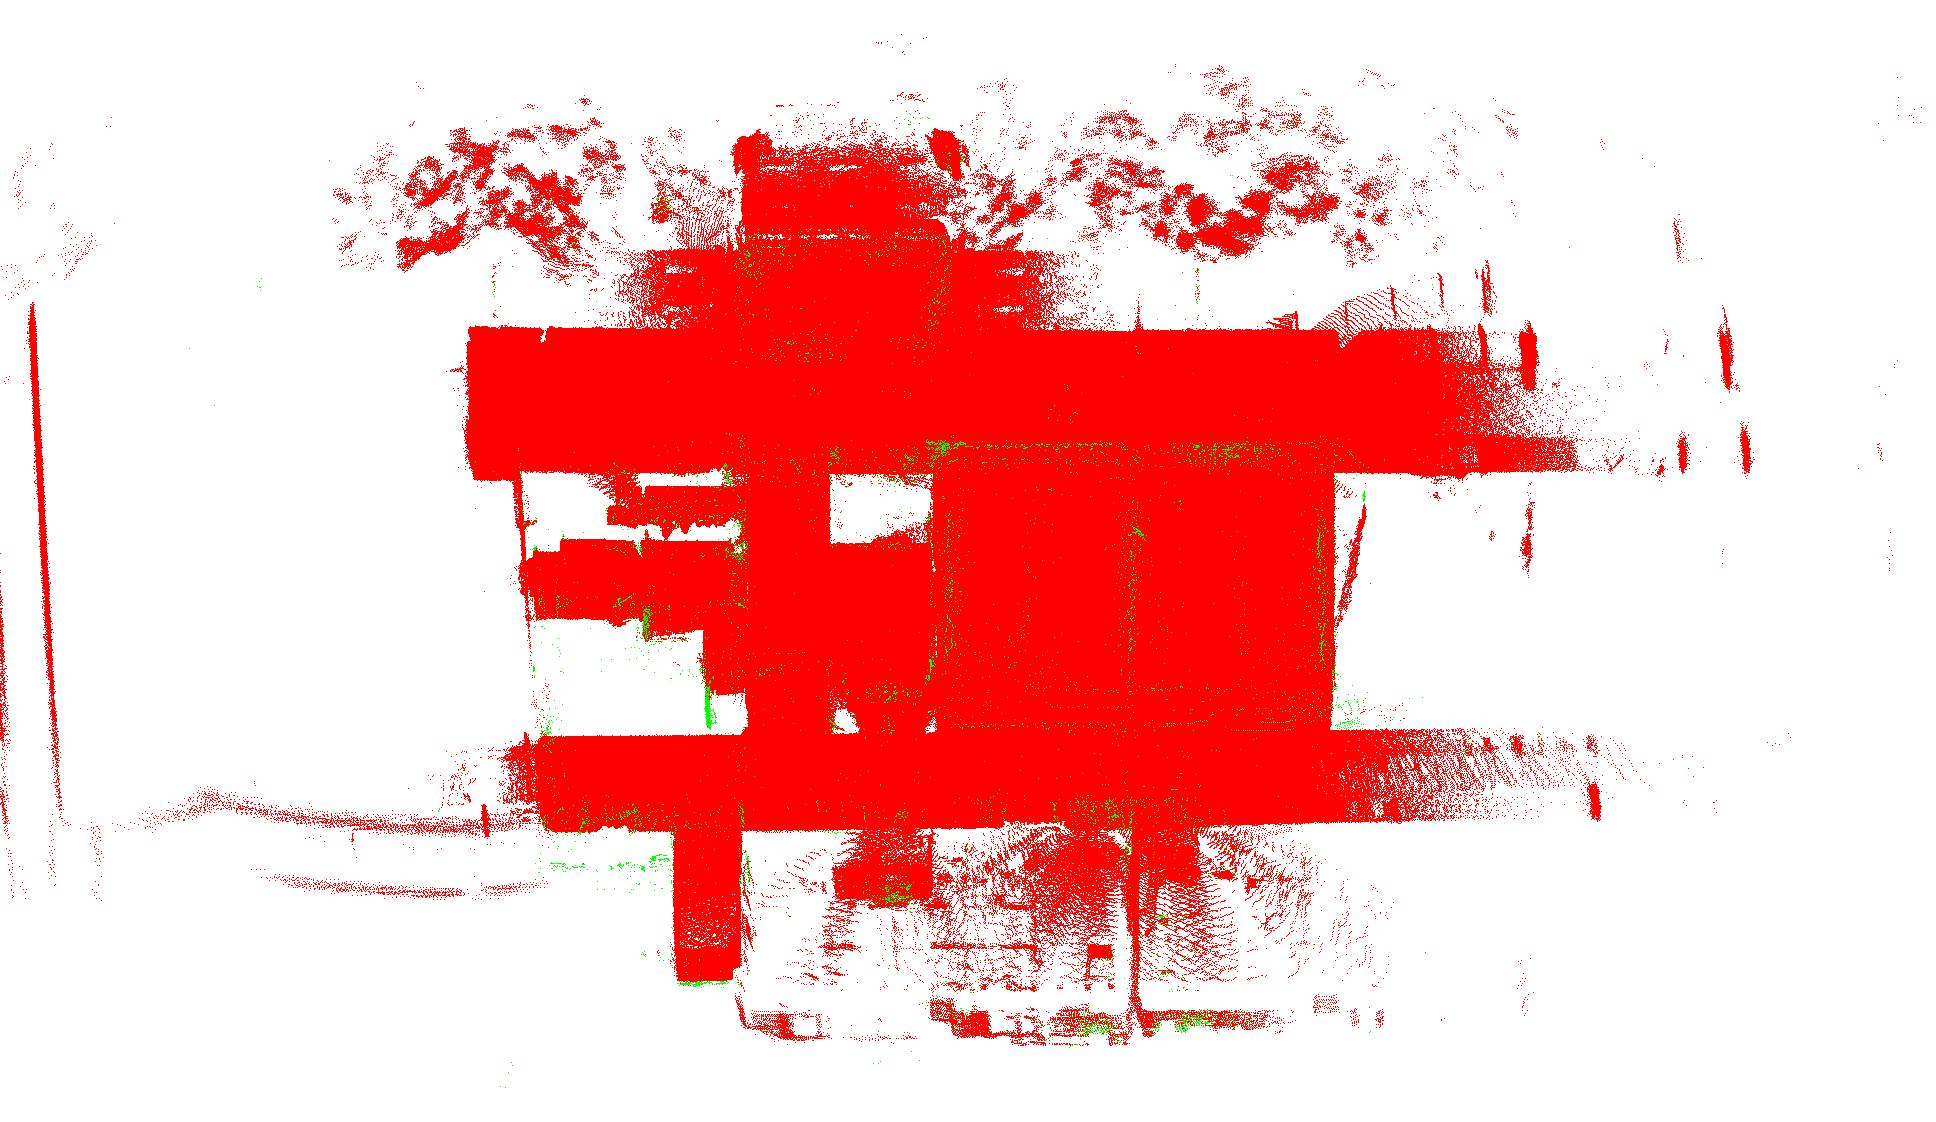}
\caption{Ouster}
\end{subfigure}

\begin{subfigure}{0.95\linewidth}
\includegraphics[width=\linewidth]{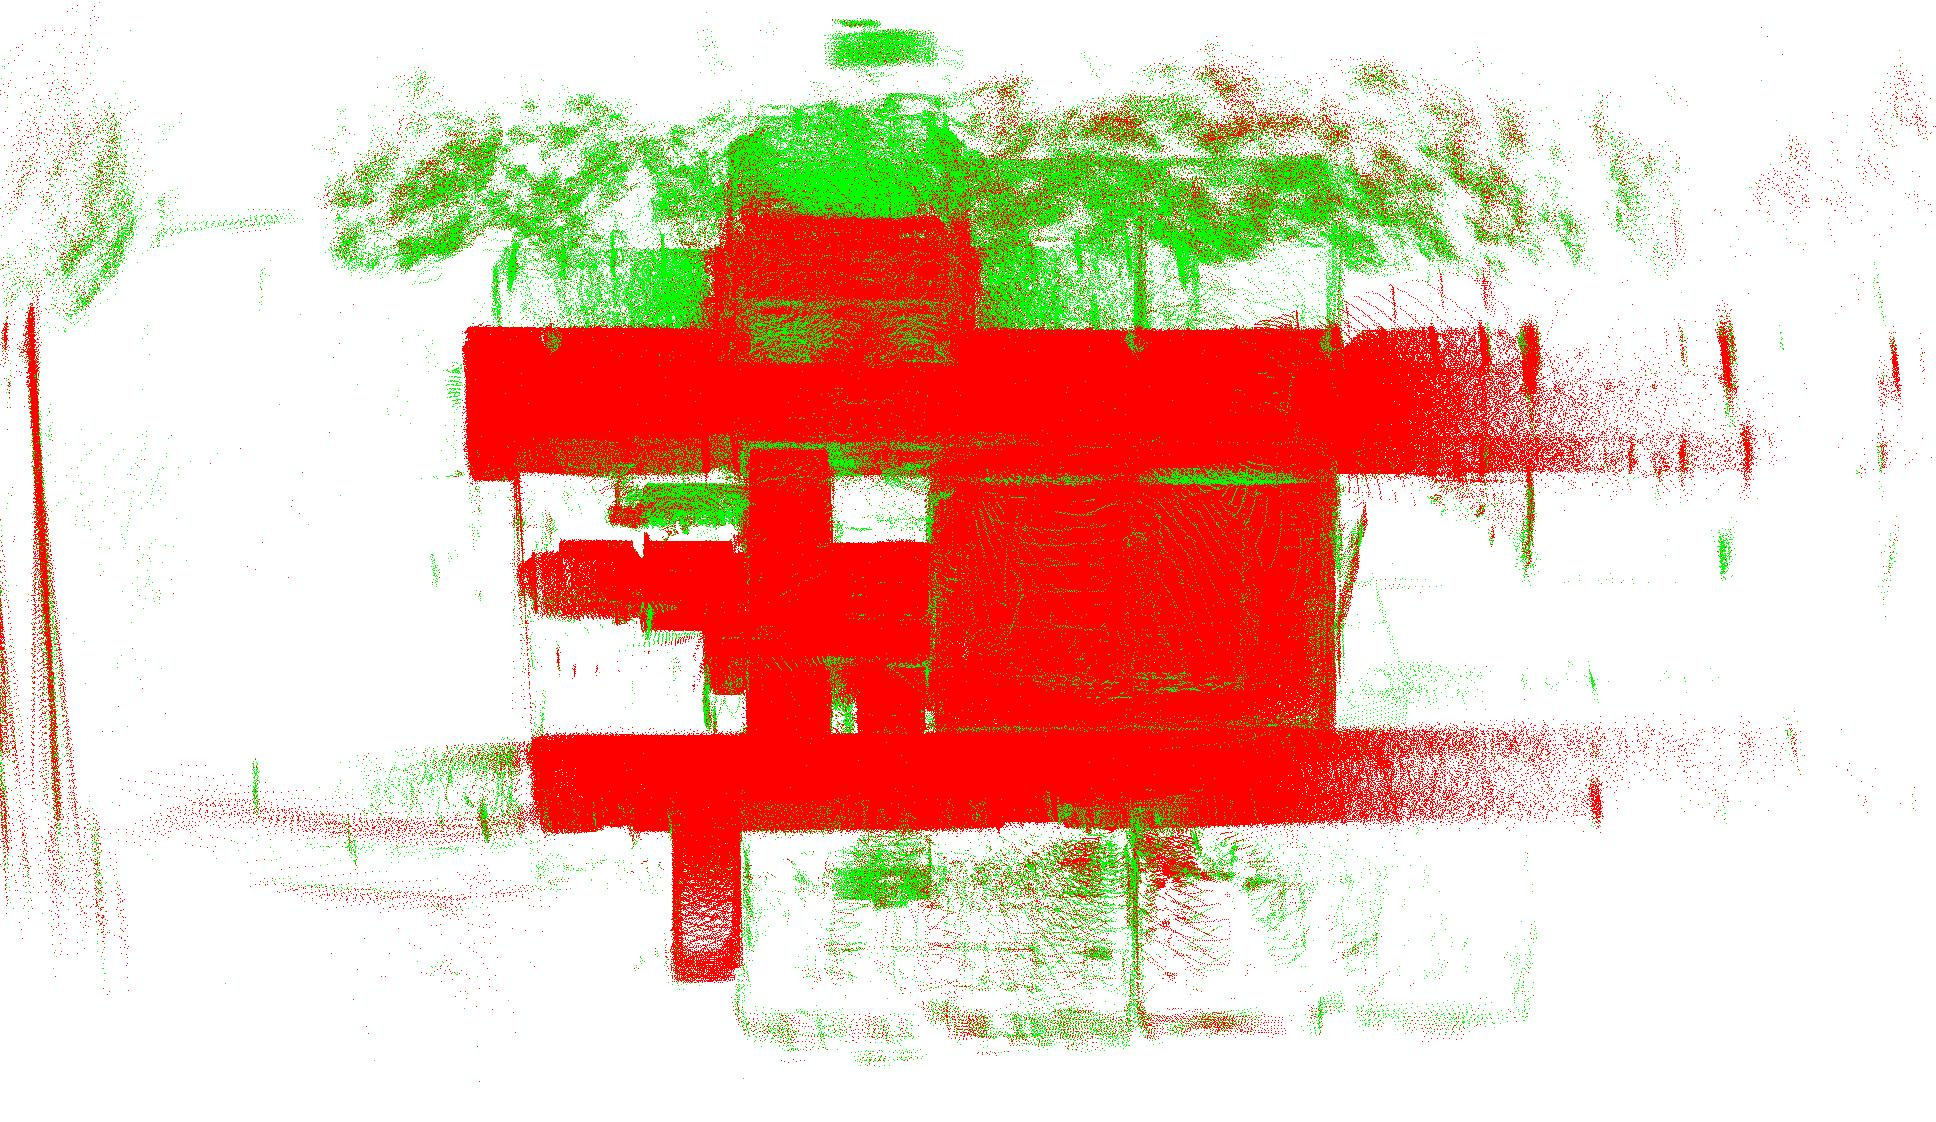}
\caption{Hesai}
\end{subfigure}
\begin{subfigure}{0.95\linewidth}
\includegraphics[width=\linewidth]{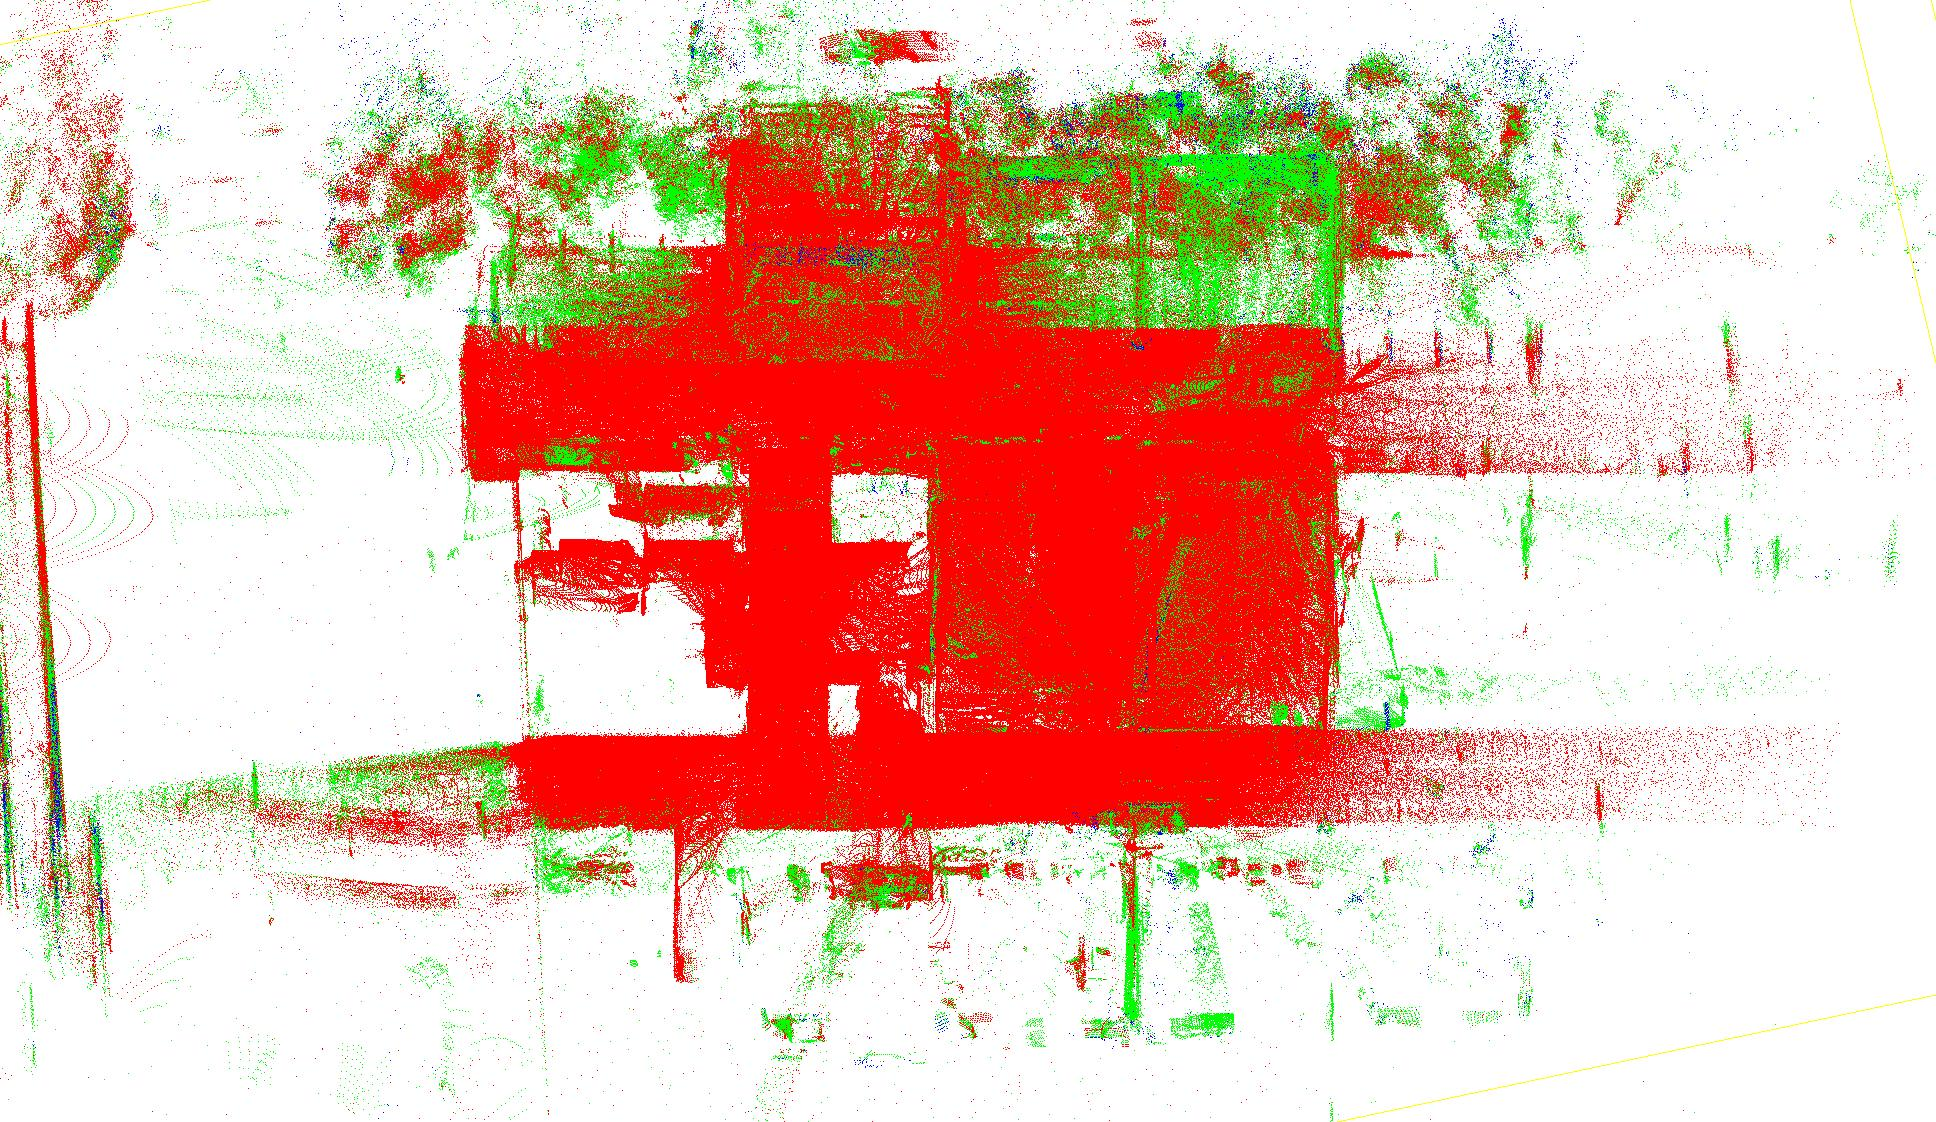}
\caption{Livox}
\end{subfigure}
\begin{subfigure}{0.95\linewidth}
\includegraphics[width=\linewidth]{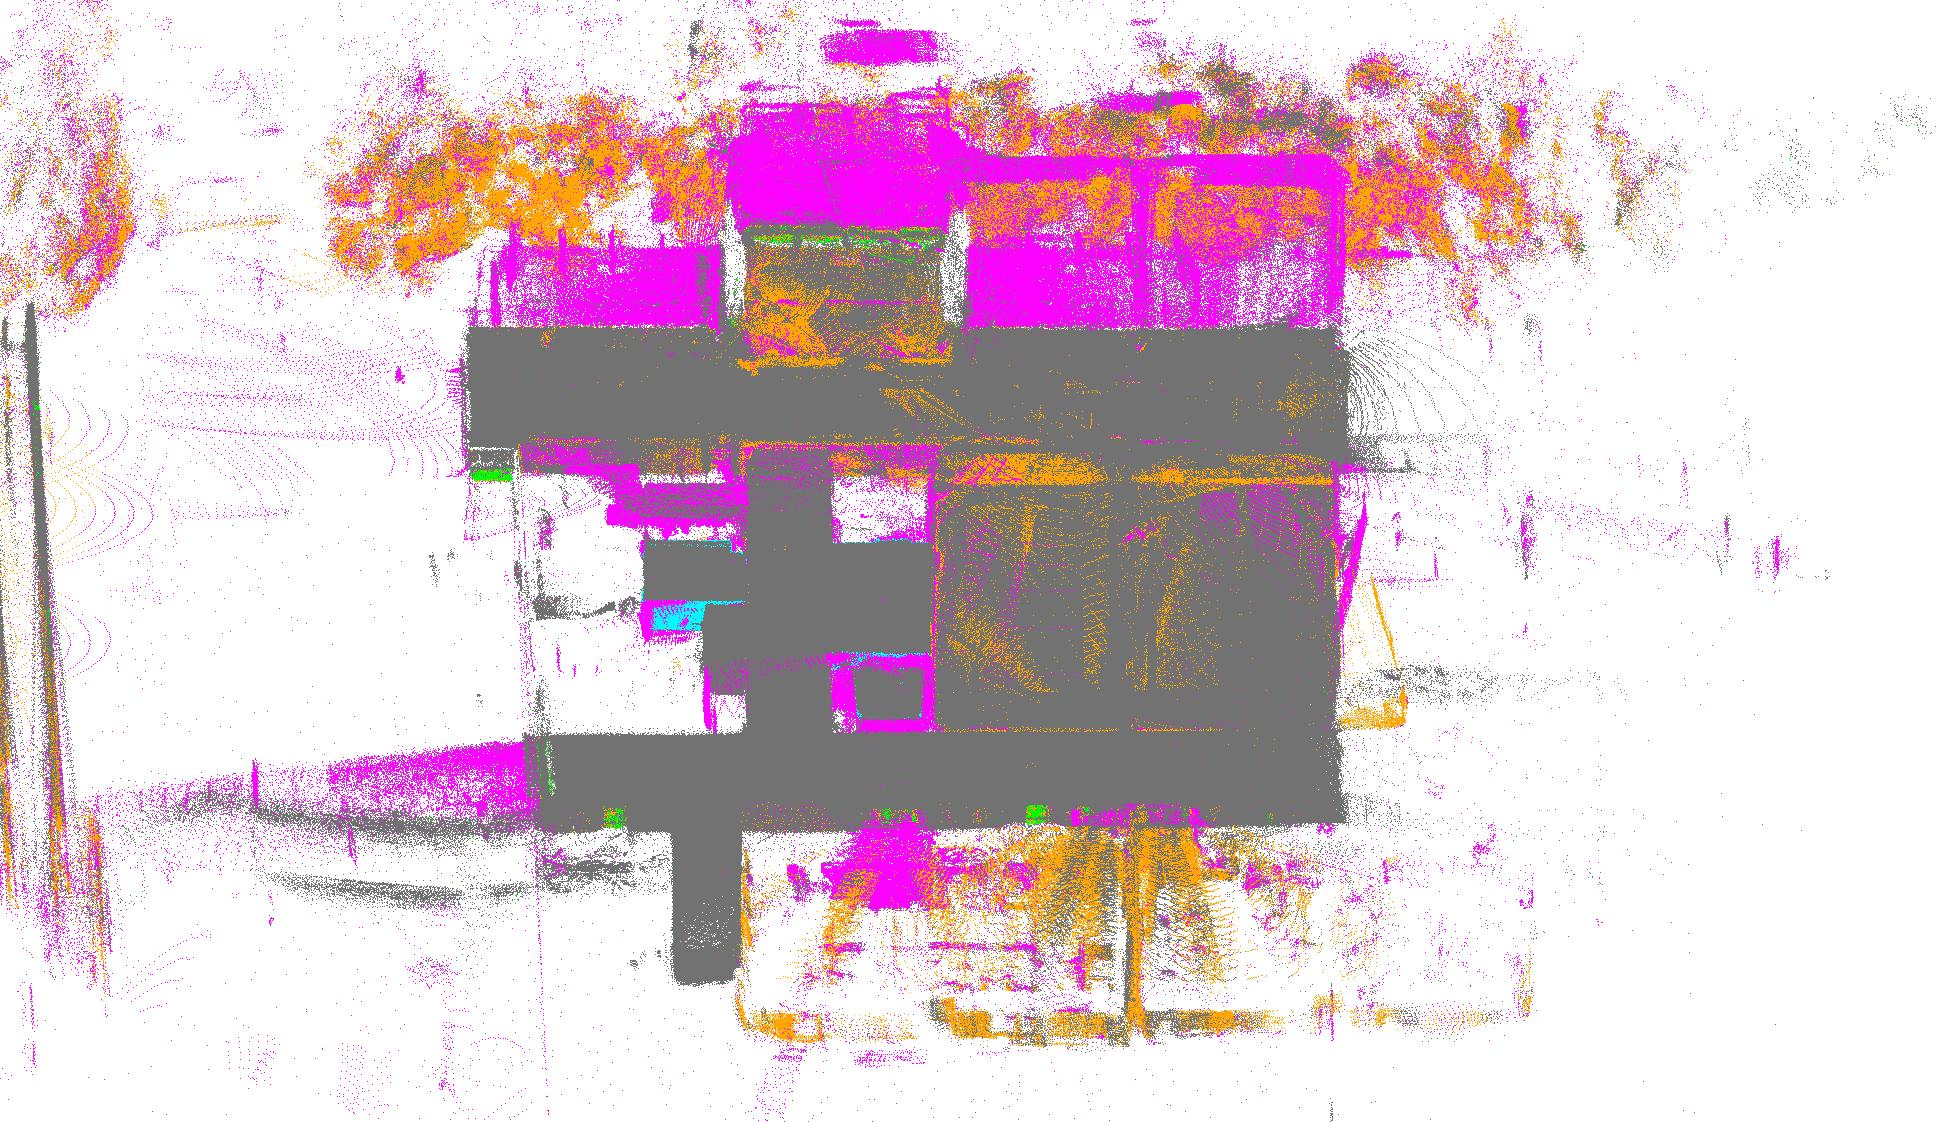}
\caption{Labels}
\end{subfigure}
\caption{Additional images from Sequence 2}
\label{fig:seq2_images}
\end{figure}

\begin{figure}[ht]
\centering

\begin{subfigure}{0.95\linewidth}
\includegraphics[width=\linewidth]{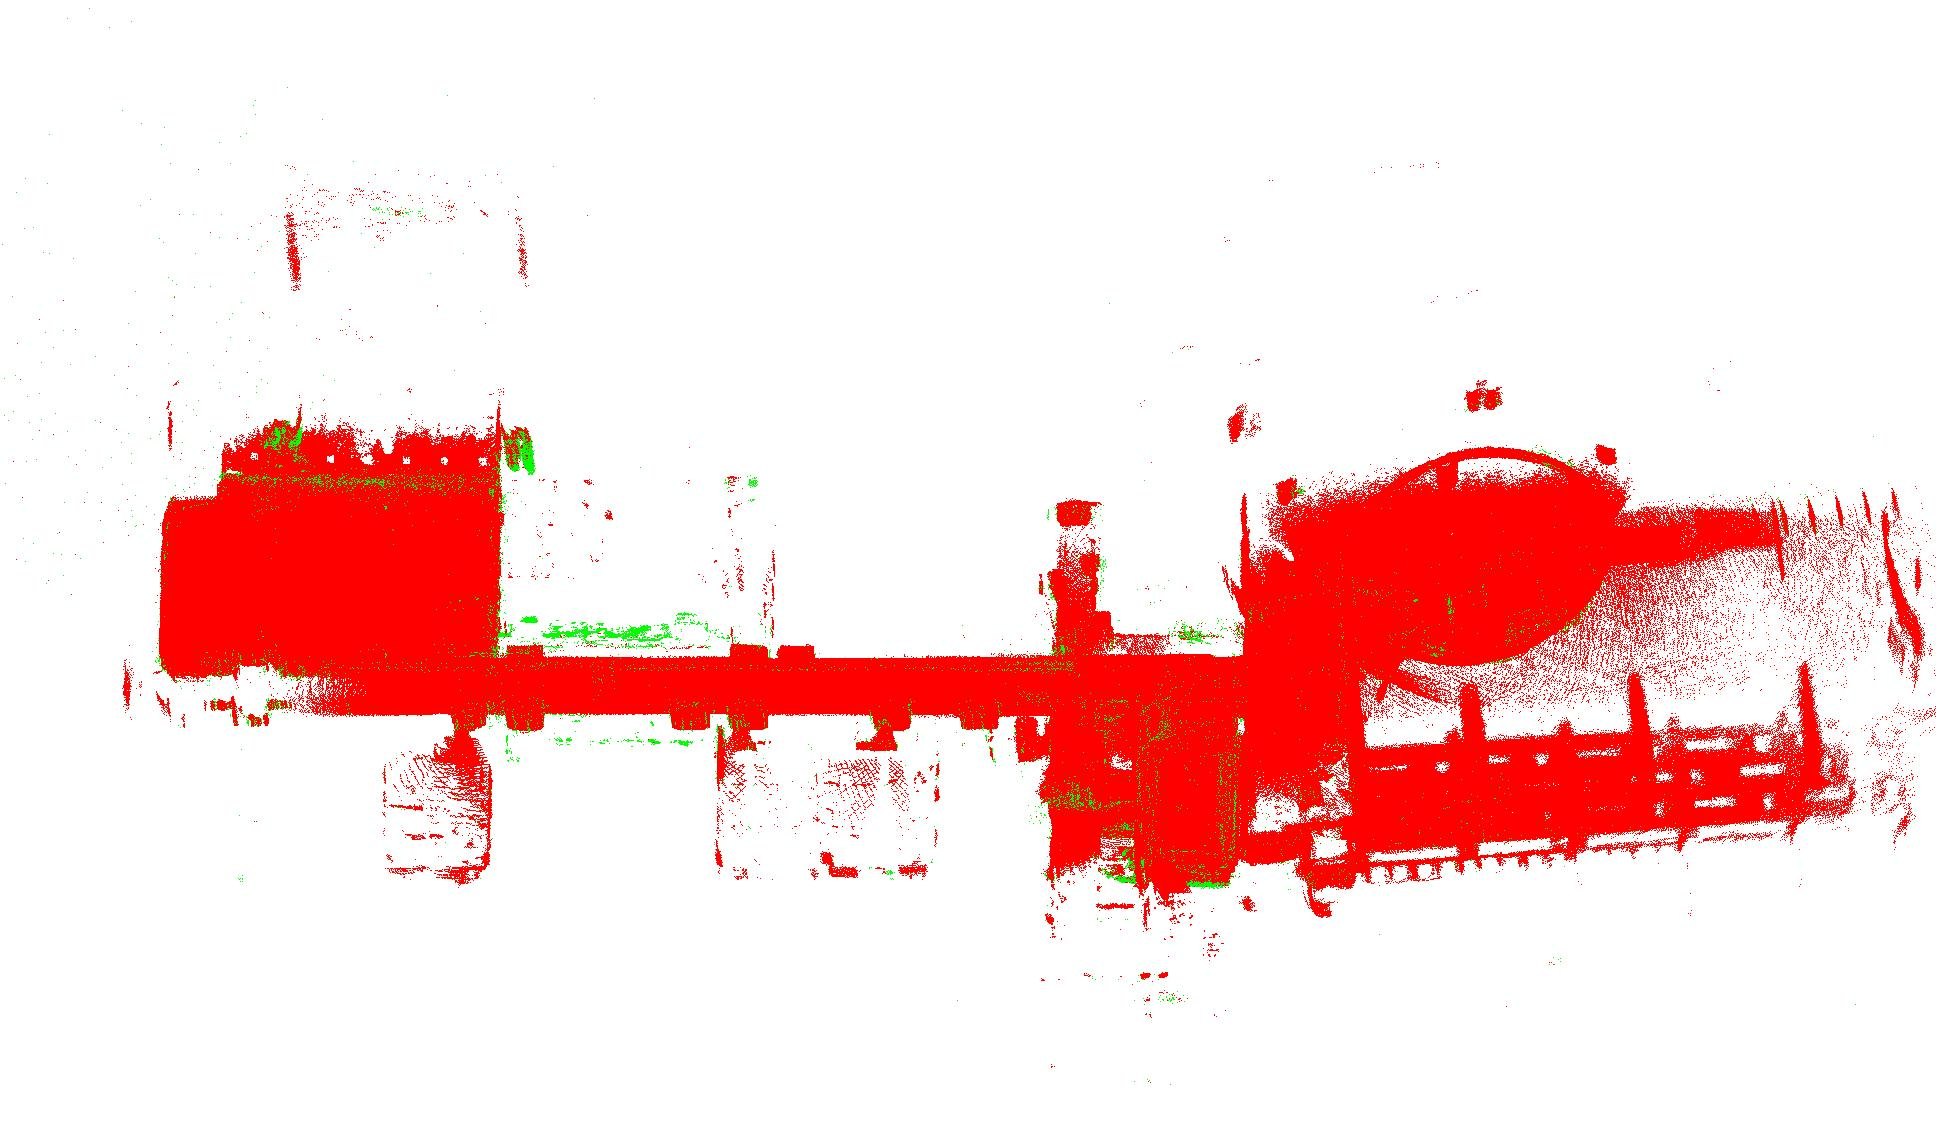}
\caption{Ouster}
\end{subfigure}
\begin{subfigure}{0.95\linewidth}
\includegraphics[width=\linewidth]{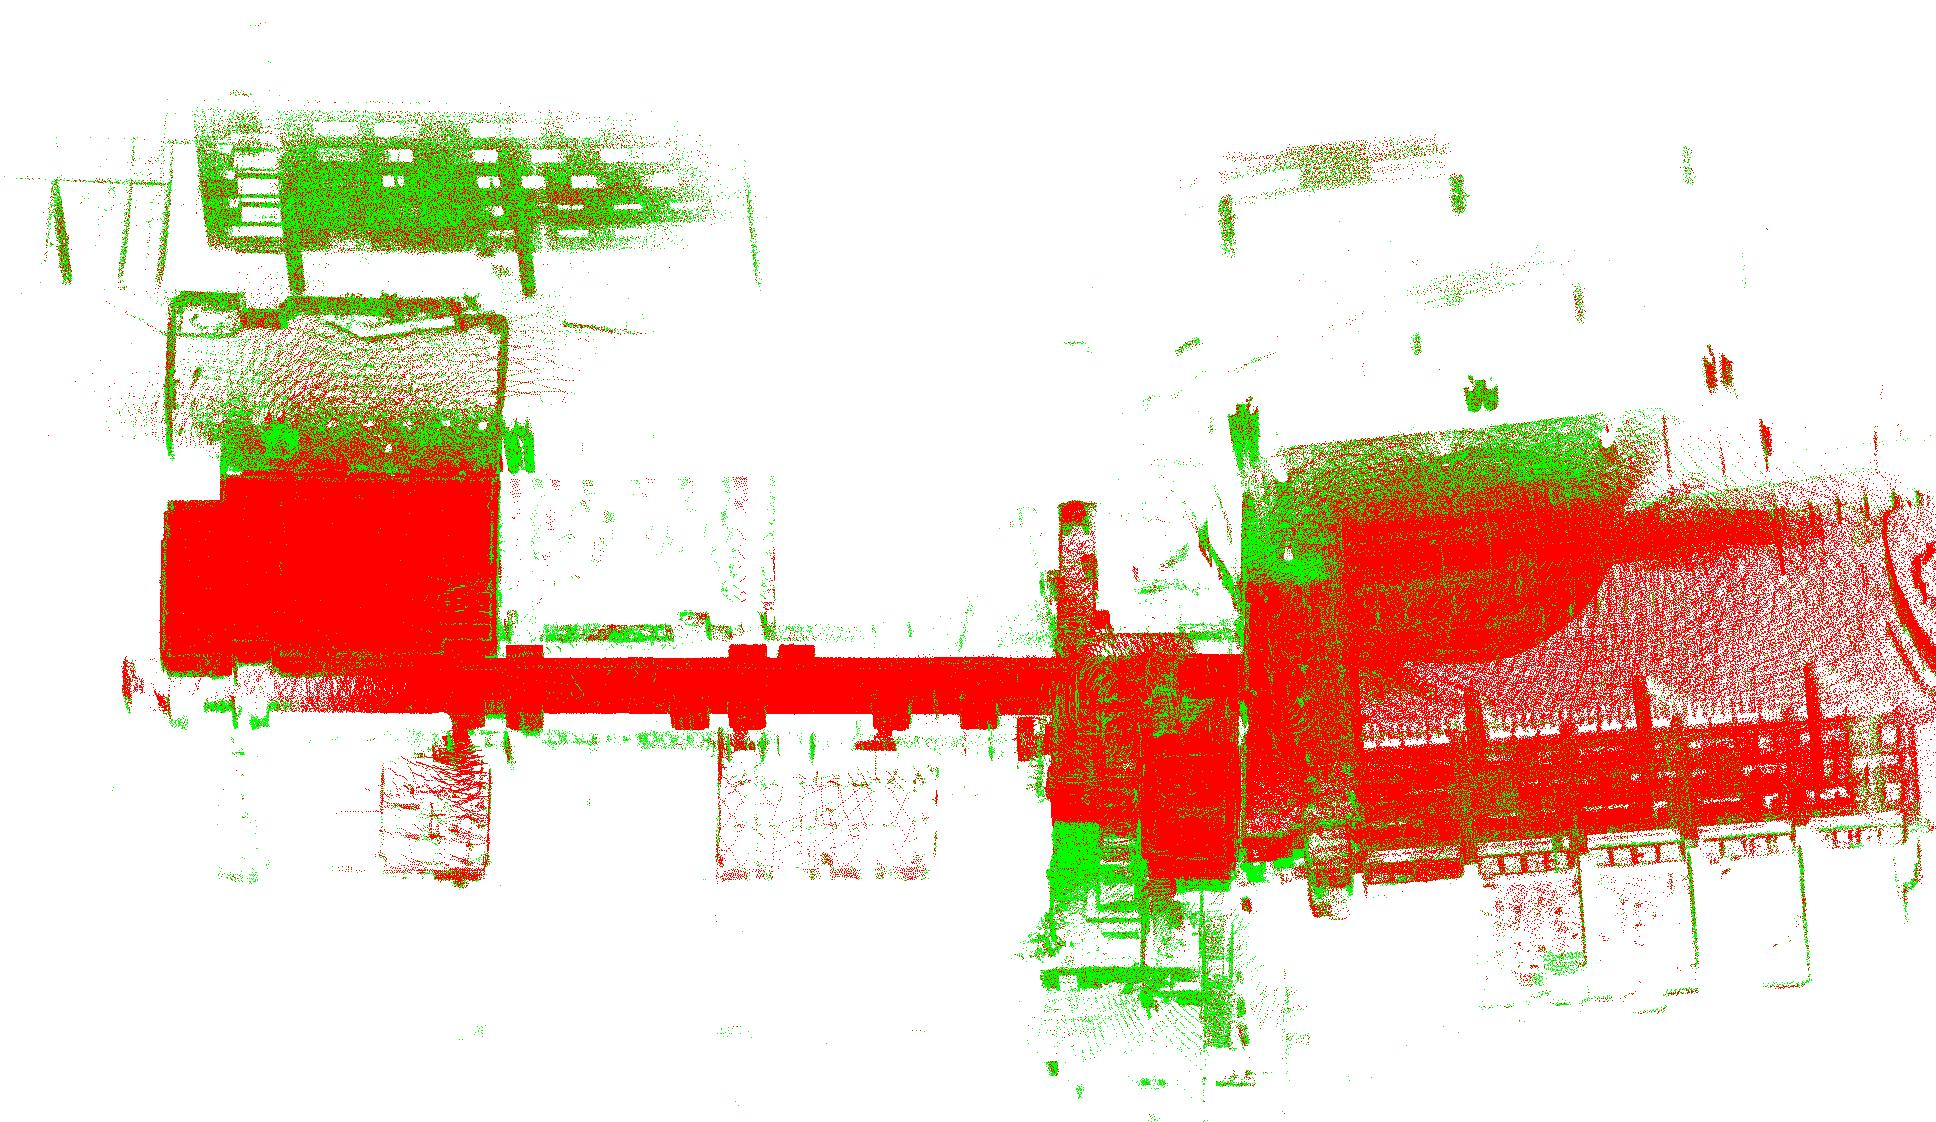}
\caption{Hesai}

\end{subfigure}
\begin{subfigure}{0.95\linewidth}
\includegraphics[width=\linewidth]{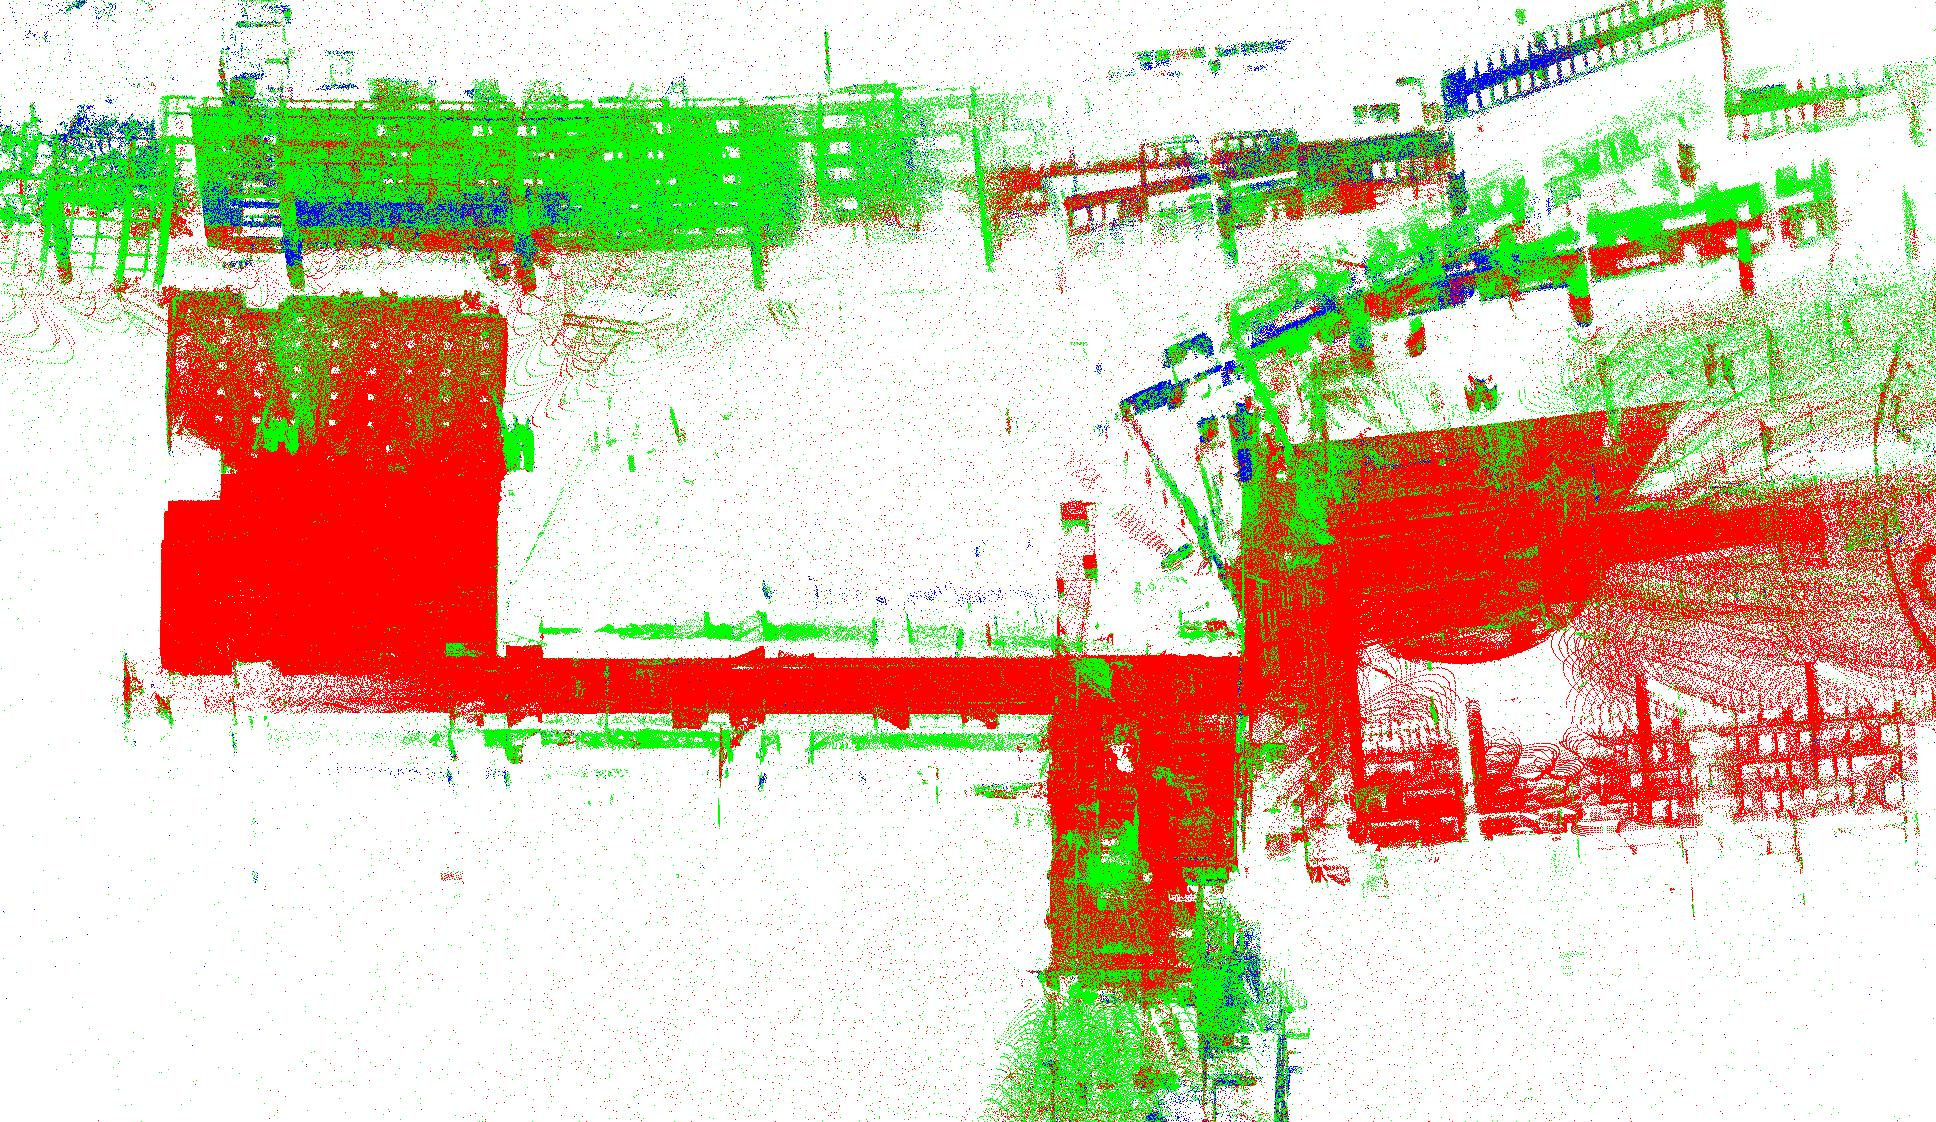}
\caption{Livox}
\end{subfigure}
\begin{subfigure}{0.95\linewidth}
\includegraphics[width=\linewidth]{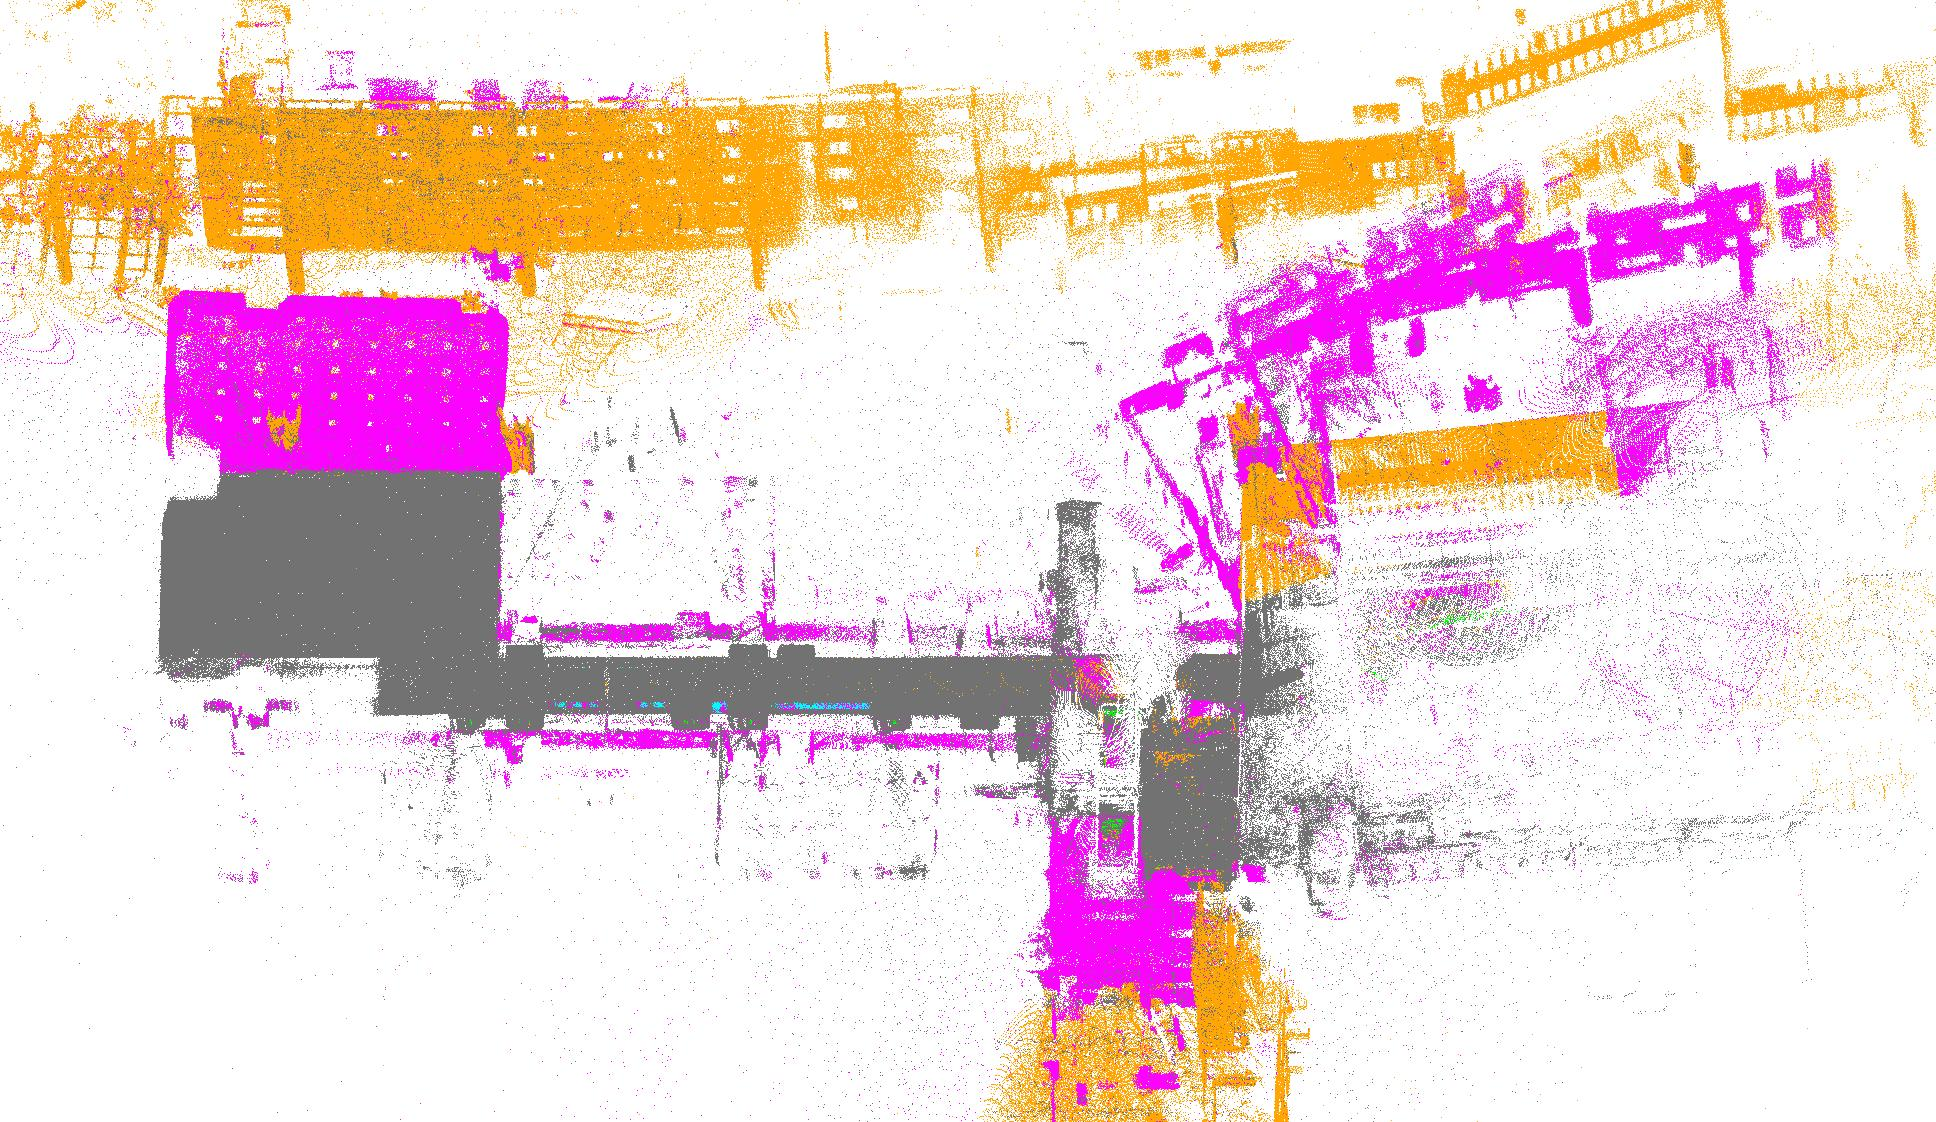}
\caption{Labels}

\end{subfigure}
\caption{Additional images from Sequence 3}
\label{fig:seq3_images}
\end{figure}

These additional visualizations further highlight the diverse reflective materials, environments, and sensor perspectives encompassed in the dataset. The multi-modal aligned data enables in-depth analysis of factors influencing reflection detection across RGB and Lidar modalities.

\subsection*{Additional Quantitative Results}

Tables \ref{tab:xyzi_confmat} and \ref{tab:xyzir_confmat} present the full confusion matrix results on per-class IoU for the Lidar methods benchmarked in the paper. Using just XYZ Intensity (Table \ref{tab:xyzi_confmat}), Cylinder3D achieves the highest reflection and obstacle points detection while SPVCNN has the best mirror and glass segmentation. Adding return information (Table \ref{tab:xyzir_confmat}) provides a small improvement, but there is still room for progress on reflections and obstacles behind glass.

Overall, these complete quantitative results demonstrate the remaining challenges and opportunities for advancing reflection analysis using multi-modal 3D data. The Lidar methods leverage geometric cues but struggle with certain reflective categories. Incorporating complementary RGB semantic information could help address these issues.

\begin{table}[b]
\centering
\caption{Confusion matrices for Lidar methods on 3DRef using XYZI}
\resizebox{\linewidth}{!}{
\begin{tabular}{l|cccccc}
\hline
& \multicolumn{6}{c}{MinkowskiNet} \\
\hline
Normal       & 98.30\% & 0.45\% & 0.05\% & 0.21\% & 0.47\% & 0.52\% \\
Glass        & 20.10\% & 78.32\% & 0.01\% & 0.01\% & 0.42\% & 1.13\% \\

Mirror       & 11.30\% & 0.02\% & 86.81\% & 0.28\% & 1.58\% & 0.00\% \\
OtherRef  & 8.52\% & 0.00\% & 0.07\% & 91.20\% & 0.20\% & 0.01\% \\
Reflection   & 2.83\% & 0.26\% & 0.16\% & 0.43\% & 91.83\% & 4.48\% \\
Obstacle     & 5.45\% & 2.08\% & 0.00\% & 0.01\% & 3.20\% & 89.26\% \\
\hline
\hline
& \multicolumn{6}{c}{SPVCNN} \\
\hline
Normal       & 98.13\% & 0.53\% & 0.05\% & 0.26\% & 0.51\% & 0.52\% \\

Glass        & 18.31\% & 79.96\% & 0.00\% & 0.00\% & 0.39\% & 1.33\% \\
Mirror       & 10.34\% & 0.03\% & 87.34\% & 0.29\% & 2.00\% & 0.01\% \\
OtherRef  & 8.09\% & 0.01\% & 0.06\% & 91.65\% & 0.19\% & 0.01\% \\
Reflection   & 2.42\% & 0.29\% & 0.13\% & 0.48\% & 93.04\% & 3.64\% \\
Obstacle     & 4.69\% & 2.05\% & 0.00\% & 0.01\% & 3.94\% & 89.32\% \\
\hline

\hline

& \multicolumn{6}{c}{Cylinder3D} \\
\hline
Normal       & 98.60\% & 0.43\% & 0.03\% & 0.21\% & 0.38\% & 0.36\% \\
Glass        & 20.65\% & 78.14\% & 0.00\% & 0.00\% & 0.31\% & 0.90\% \\
Mirror       & 12.12\% & 0.02\% & 86.09\% & 0.34\% & 1.42\% & 0.00\% \\
OtherRef  & 10.11\% & 0.00\% & 0.02\% & 89.72\% & 0.15\% & 0.00\% \\
Reflection   & 2.26\% & 0.27\% & 0.14\% & 0.38\% & 94.51\% & 2.44\% \\

Obstacle     & 4.39\% & 1.80\% & 0.00\% & 0.00\% & 2.11\% & 91.70\% \\
\hline
\end{tabular}
}
\label{tab:xyzi_confmat}
\end{table}

\begin{table}[b]
\centering
\caption{Confusion matrices for Lidar methods on 3DRef using XYZIR}
\resizebox{\linewidth}{!}{
\begin{tabular}{l|cccccc}
\hline
& \multicolumn{6}{c}{MinkowskiNet} \\
\hline
Normal       & 98.29\% & 0.50\% & 0.06\% & 0.22\% & 0.45\% & 0.47\% \\
Glass        & 18.28\% & 80.36\% & 0.03\% & 0.00\% & 0.28\% & 1.05\% \\
Mirror       & 10.81\% & 0.02\% & 87.37\% & 0.25\% & 1.54\% & 0.00\% \\
Other Refl.  & 8.44\% & 0.00\% & 0.07\% & 91.32\% & 0.16\% & 0.00\% \\
Reflection   & 2.36\% & 0.27\% & 0.17\% & 0.35\% & 93.60\% & 3.25\% \\
Obstacle     & 4.34\% & 2.14\% & 0.00\% & 0.00\% & 3.06\% & 90.45\% \\
\hline
\hline
& \multicolumn{6}{c}{SPVCNN} \\
\hline

Normal       & 98.18\% & 0.53\% & 0.05\% & 0.22\% & 0.50\% & 0.52\% \\
Glass        & 18.56\% & 79.91\% & 0.01\% & 0.00\% & 0.33\% & 1.20\% \\
Mirror       & 10.15\% & 0.03\% & 87.60\% & 0.39\% & 1.84\% & 0.01\% \\
Other Refl.  & 6.43\% & 0.01\% & 0.05\% & 93.32\% & 0.19\% & 0.01\% \\
Reflection   & 2.30\% & 0.34\% & 0.16\% & 0.41\% & 92.81\% & 3.97\% \\
Obstacle     & 4.51\% & 2.29\% & 0.00\% & 0.01\% & 3.56\% & 89.64\% \\
\hline
\hline
& \multicolumn{6}{c}{Cylinder3D} \\
\hline
Normal       & 98.62\% & 0.45\% & 0.03\% & 0.21\% & 0.35\% & 0.33\% \\

Glass        & 19.88\% & 79.00\% & 0.00\% & 0.00\% & 0.24\% & 0.89\% \\
Mirror       & 11.41\% & 0.02\% & 86.82\% & 0.32\% & 1.43\% & 0.00\% \\
Other Refl.  & 10.41\% & 0.00\% & 0.02\% & 89.44\% & 0.12\% & 0.00\% \\
Reflection   & 2.19\% & 0.26\% & 0.14\% & 0.29\% & 94.86\% & 2.26\% \\

Obstacle     & 4.19\% & 1.86\% & 0.00\% & 0.00\% & 2.02\% & 91.92\% \\
\hline
\end{tabular}
}
\label{tab:xyzir_confmat}
\end{table}

\subsection*{Additional RGB Results}

Figure \ref{fig:rgb_results} shows sample semantic segmentation results on RGB images after retraining the EBLNet model on all reflection labels in the 3DRef dataset. The predicted masks are visualized overlayed on the original images.

\begin{figure}[htbp]
\centering
\begin{subfigure}{0.45\linewidth}
\includegraphics[width=\linewidth]{supplresult/origin (1).png}
\end{subfigure}
\begin{subfigure}{0.45\linewidth}
\includegraphics[width=\linewidth]{supplresult/masknew (1).png}
\end{subfigure}
\begin{subfigure}{0.45\linewidth}
\includegraphics[width=\linewidth]{supplresult/origin (2).png}
\end{subfigure}
\begin{subfigure}{0.45\linewidth}
\includegraphics[width=\linewidth]{supplresult/masknew (2).png}
\end{subfigure}
\begin{subfigure}{0.45\linewidth}
\includegraphics[width=\linewidth]{supplresult/origin (3).png}
\end{subfigure}
\begin{subfigure}{0.45\linewidth}
\includegraphics[width=\linewidth]{supplresult/masknew (3).png}
\end{subfigure}
\begin{subfigure}{0.45\linewidth}
\includegraphics[width=\linewidth]{supplresult/origin (4).png}
\end{subfigure}
\begin{subfigure}{0.45\linewidth}
\includegraphics[width=\linewidth]{supplresult/masknew (4).png}
\end{subfigure}
\begin{subfigure}{0.45\linewidth}
\includegraphics[width=\linewidth]{supplresult/origin (5).png}
\end{subfigure}
\begin{subfigure}{0.45\linewidth}
\includegraphics[width=\linewidth]{supplresult/masknew (5).png}
\end{subfigure}
\begin{subfigure}{0.45\linewidth}
\includegraphics[width=\linewidth]{supplresult/origin (6).png}
\end{subfigure}
\begin{subfigure}{0.45\linewidth}
\includegraphics[width=\linewidth]{supplresult/masknew (6).png}
\end{subfigure}
\caption{Additional RGB results with EBLNet retrained on 3DRef (left column are origin images and right column are image covered with mask from retrained EBLNet)}
\label{fig:rgb_results}
\end{figure}

These examples illustrate the robust reflection detection achieved by retraining on the diverse 3DRef data. The network generalizes well to various materials, surfaces, and environments. However, some failure cases still arise, presenting opportunities for further progress. The additional RGB results confirm the benefits of multi-modal aligned training data for reflection segmentation.

\clearpage

\subsection*{Dataset Format}
In the supplementary matertial we provide a folder of dataset sample, which shows the dataset format. We describe the dataset format in the following.
\begin{itemize}
\item \texttt{raw}: Contains the raw sensor data for each sequence, including pose files, images, meshes, raycast point clouds, and more. Each sequence is in a separate subfolder.
\begin{itemize}
\item \texttt{seq1}
\begin{itemize}

\item \texttt{hesai\_pose.txt}
\item \texttt{images}
\item \texttt{livox\_pose.txt}
\item \texttt{mesh}
\item \texttt{ouster\_pose.txt}
\item \texttt{raycast}
\begin{itemize}
\item \texttt{hesai}
\item \texttt{livox}
\item \texttt{ouster}

\end{itemize}
\item \texttt{vo\_kf.txt}
\end{itemize}
\item \texttt{seq2}, \texttt{seq3}, \ldots
\end{itemize}

\item \texttt{rgb}: Folder for RGB images and masks split into train/test folders for each label type (glass, mirror, other reflective, all reflective). Images and masks are paired in separate subfolders.
\begin{itemize}
\item \texttt{alllabel}
\begin{itemize}
\item \texttt{test}
\begin{itemize}

\item \texttt{image}
\item \texttt{mask}
\end{itemize}
\item \texttt{train}
\begin{itemize}
\item \texttt{image}
\item \texttt{mask}
\end{itemize}
\end{itemize}
\item \texttt{glass}, \texttt{mirror}, \texttt{otherref}, \ldots
\end{itemize}

\item \texttt{script}: Helper scripts for dataset processing.

\item \texttt{semantickitti}: Labeled Lidar point clouds in SemanticKitti format, with separate folders for XYZI and XYZIR channels. Point clouds for each sequence are under \texttt{sequences/00/velodyne}.

\item \texttt{network}: Source code and pretrained weights for reflection detection networks like EBLNet, PCSeg, and SATNet.

\end{itemize}

The \texttt{raw} folder contains the core data needed to recreate the annotations and formatted dataset. The \texttt{rgb} and \texttt{semantickitti} folders provide the formatted data split into train/test sets ready for benchmarking. The \texttt{network} folder enables out-of-the-box evaluation using provided models. Refer to the readme for additional details.

\section*{Conclusion}

These supplementary materials provide additional results and dataset details to complement the core paper. The visualizations showcase the data diversity. The full confusion matrices highlight remaining segmentation challenges. The dataset structure facilitates access for further research. Please refer to the main paper for an in-depth discussion of the 3DRef contributions.
